# Supplementary material for: Nanoscale Protein Diffusion in Supercooled Cryoprotectant Solutions
Source: arXiv:2512.02742 ancillary file (2026-07-13)
Supplement: Supplementary file 1 [file SI.pdf]

## Supporting Information:

# Protein Diffusion and Stokes–Einstein Deviation in Supercooled Cryoprotectant Solutions

Maddalena Bin,<sup>†</sup> Anita Girelli,<sup>†,‡</sup> Mariia Filianina,<sup>†</sup> Mario Reiser,<sup>†</sup> Sharon Berkowicz,<sup>†</sup> Milla  
Åhlfeldt,<sup>†</sup> Michelle Dargasz,<sup>¶</sup> Sonja Timmermann,<sup>¶</sup> Jaqueline Savelkoul,<sup>§</sup> Takeshi Kawasaki,<sup>||,⊥</sup>  
Shinji Saito,<sup>#,®</sup> Federico Zontone,<sup>△</sup> Yuriy Chushkin,<sup>△</sup> Fajun Zhang,<sup>‡</sup> Frank Schreiber,<sup>‡</sup> Michael  
Paulus,<sup>▽</sup> Christian Gutt,<sup>¶</sup> and Fivos Perakis\*,<sup>†</sup>

<sup>†</sup>*Department of Physics, AlbaNova University Center, Stockholm University, S-106 91  
Stockholm, Sweden*

<sup>‡</sup>*Institut für Angewandte Physik, Universität Tübingen, Auf der Morgenstelle 10, 72076  
Tübingen, Germany*

<sup>¶</sup>*Department Physik, Universität Siegen, Walter-Flex-Strasse 3, 57072, Siegen, Germany*

<sup>§</sup>*Fakultät Physik/DELTA, TU Dortmund, Maria-Goeppert-Mayer-Str. 2, 44221 Dortmund,  
Germany*

<sup>||</sup>*D3 Center, The University of Osaka, Toyonaka, Osaka, 560-0043, Japan*

<sup>⊥</sup>*Department of Physics, The University of Osaka, Toyonaka, Osaka, 560-0043, Japan*

<sup>#</sup>*Institute for Molecular Science, Myodaiji, Okazaki, Aichi 444-8585, Japan*

<sup>®</sup>*The Graduate University for Advanced Studies (SOKENDAI), Myodaiji, Okazaki, Aichi  
444-8585, Japan*

<sup>△</sup>*ESRF - The European Synchrotron, 71 Avenue des Martyrs, Grenoble, 38000, France*

<sup>▽</sup>*Fakultät Physik/DELTA, TU Dortmund, 44221 Dortmund, Germany*

E-mail: f.perakis@fysik.su.se

# Intensity autocorrelation function - $q$ -dependence

## Single exponential

The intensity autocorrelation functions  $g_2(q, t)$ , displayed in Fig.S1a-e, for ferritin solutions at different momentum transfer  $q$  and temperatures  $T = 210 - 250$  K. The  $g_2(q, t)$  functions are fitted with a simple exponential function (solid lines). The decorrelation rate  $\Gamma(q)$  in Fig. S1f exhibits the  $q^2$ -dependance of the diffusion coefficient  $D$  and the solid line depicts the fit by  $\Gamma(q) = D q^2$ . The quadratic fit describes well the data for the probed  $q$ -range.

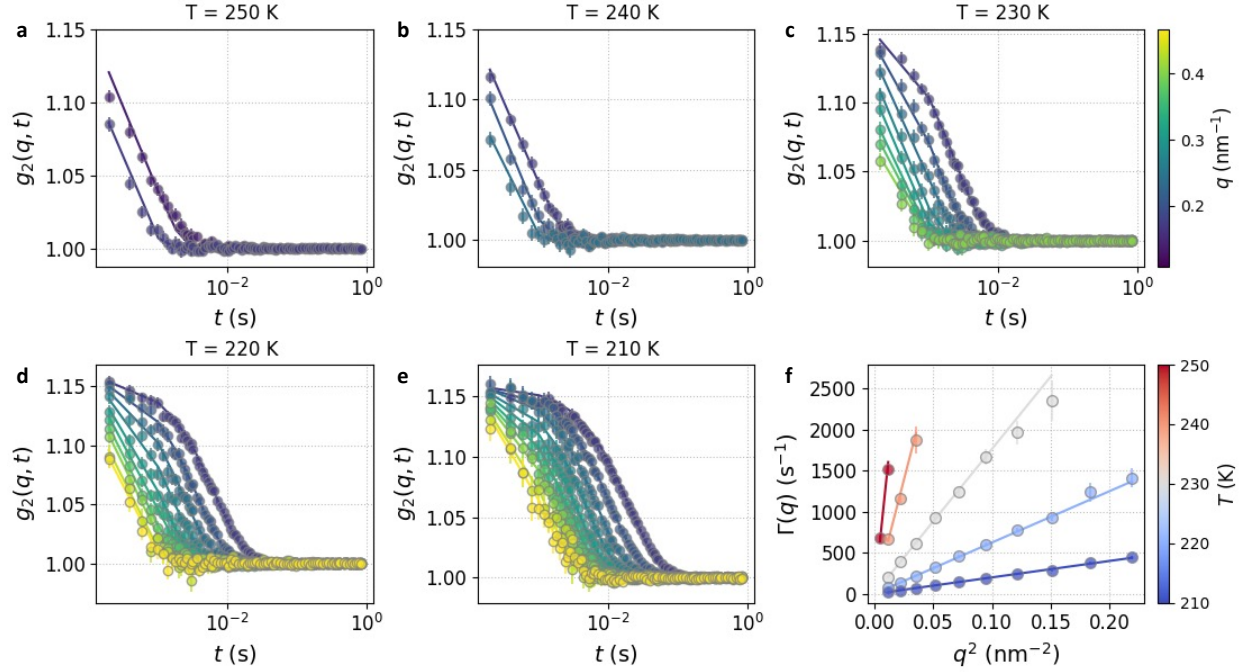

Fig. S1:  $q$ -dependence of intensity autocorrelation functions of ferritin solutions. (a)-(e) Intensity autocorrelation functions  $g_2(q, t)$  for different momentum transfer  $q$ -values and different temperatures  $T = 210 - 250$  K, fitted with a simple exponential function (solid lines). (f) Decorrelation time  $\Gamma(q)$  extracted from the fits of the  $g_2(q, t)$  functions in panels a-e, shown as a function of the squared momentum transfer  $q^2$  along with a linear fit (solid line).

## Stretched exponential

We fit the intensity autocorrelation functions with a stretched exponential  $g_2(q, t) = \beta \exp [-(2t \Gamma(q))^\alpha]$ , where  $\alpha$  is the Kohlrausch-Williams-Watts (KWW) exponent. The result is shown in Fig. S2.

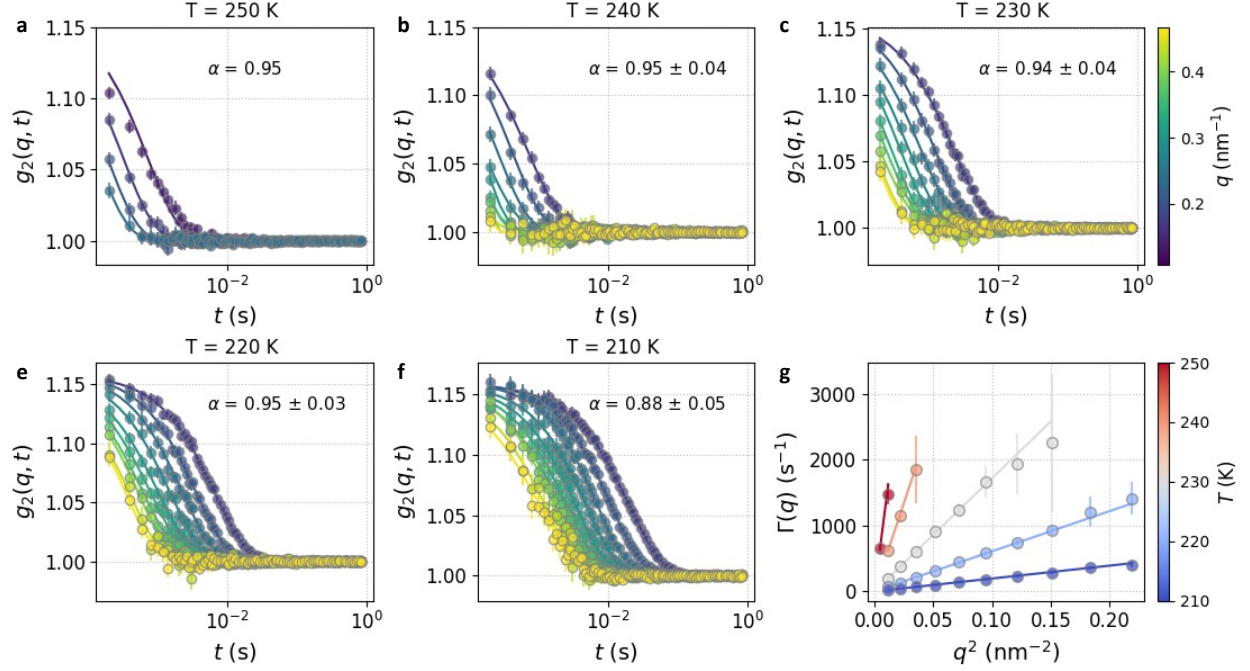

Fig. S2:  $q$ -dependence of intensity autocorrelation functions of ferritin solutions. (a)-(e) Intensity autocorrelation functions  $g_2(q, t)$  for different momentum transfer  $q$ -values and different temperatures  $T = 210 - 250$  K, fitted with a stretched exponential function, which includes the KWW exponent (solid lines). (f) KWW exponent as a function of  $q$ , extracted from the fit of the  $g_2(q, t)$  functions in panels a-e.

## Silica nanoparticles

The intensity autocorrelation functions  $g_2(q, t)$ , displayed in Fig.S3 a-e, for silica nanoparticle solutions ( $R_h = 50$  nm) at  $q = 0.01 - 0.05$  nm<sup>-1</sup> and temperatures  $T = 200 - 270$  K. The  $g_2(q, t)$  functions are fitted with a simple exponential function (solid lines). The decorrelation rate  $\Gamma(q)$  in Fig. S3h exhibits the  $q^2$ -dependence of the diffusion coefficient  $D$  and the solid line depicts the fit by  $\Gamma(q) = D q^2$ . The quadratic fit describes well the data for the probed  $q$ -range.

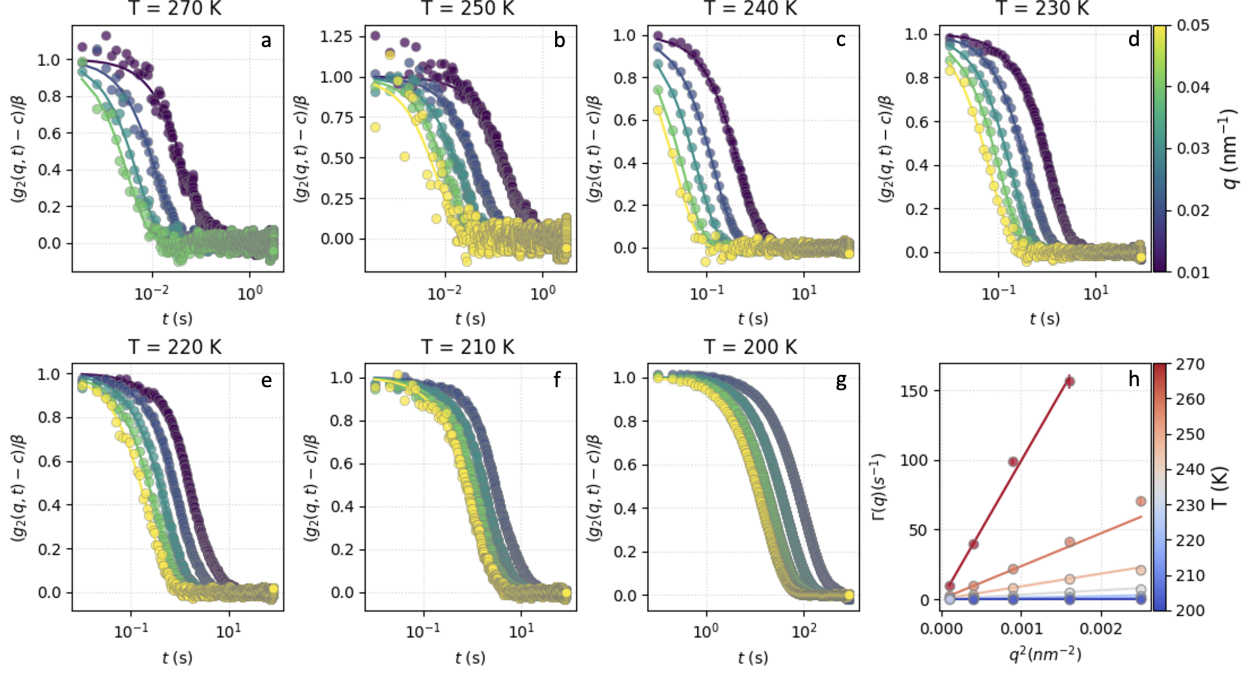

Fig. S3:  $q$ -dependence of intensity autocorrelation functions of silica nanoparticle solutions. (a-g) Panels depict the intensity autocorrelation functions  $g_2(q, t)$  for different momentum transfer  $q$ -values and different temperatures  $T = 200\text{--}270$  K, fitted with a simple exponential function (solid lines). (h) Decorrelation time  $\Gamma(q)$  extracted from the fits of the  $g_2(q, t)$  functions in panels a-e, shown as a function of the squared momentum transfer  $q^2$  along with a linear fit (solid line).

## Hydrodynamic radius estimation from DLS

The protein diffusion coefficient  $D_0$  was measured at dilute conditions ( $c = 9$  mg/ml) at 298 K using DLS. The LS spectrometer used is from LS Instruments AG equipped with a  $\lambda = 660$  nm CW laser. The computed  $g_2$  functions are reported in Fig. S4a. The decorrelation rate  $\Gamma(q)$  was extracted by fitting a simple exponential decay, with the expression  $g_2(q, t) = \beta \exp[-2t\Gamma(q)] - 1$ . The extracted decorrelation rates are shown in Fig. S4b. A hydrodynamic radius of  $R_h = 7.2$  nm was determined by the Stokes-Einstein relation.

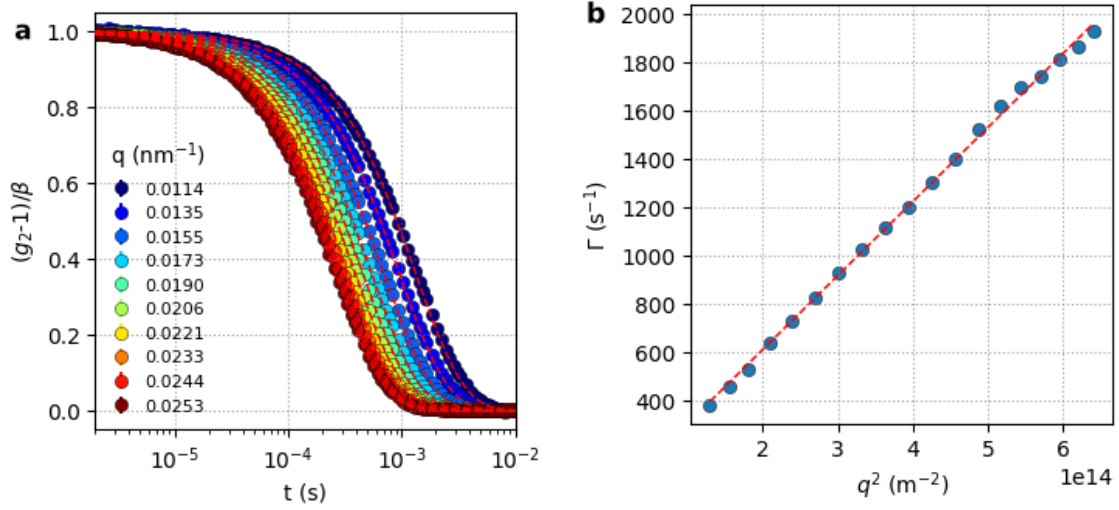

Fig. S4: Dynamic light scattering (DLS) measurements of ferritin solutions. The data shown correspond to dilute condition ( $c = 9$  mg/ml) in water-glycerol (with glycerol 23 mol%). (a) The intensity autocorrelation function,  $g_2(q, t)$ , is shown for different  $q$ -values, as indicated in the legend. The  $g_2(q, t)$  is normalised by the corresponding speckle contrast. (b) The extracted decorrelation rate  $\Gamma(q)$  obtained from the  $g_2(q, t)$  using an exponential fit. The solid line is a linear fit and the slope gives the diffusion coefficient  $D_0$  in the dilute limit.

## Intensity autocorrelation function - Flux Dependence

Identifying the onset of X-ray beam-induced effects is crucial for performing XPCS in soft biological matter. Beam-induced effects can manifest as flux-dependent changes in the scattering intensity  $I(q)$  or in the corresponding dynamics. Dynamics are particularly sensitive to any beam-induced effects, as they can reflect acceleration due to local fluidization<sup>1</sup> and radiolysis,<sup>2</sup> or alternatively gradual deceleration due to beam-induced aggregation.<sup>3</sup>

We performed flux-dependent XPCS measurements of ferritin solutions in water-glycerol (see Methods section) to identify the conditions under which any X-ray beam effects were negligible. Fig. S5a shows the  $g_2(q, t)$  at momentum transfer  $q = 0.1$  nm<sup>-1</sup> and temperature  $T = 220$ K, for three different flux conditions, ranging from  $F = 1.6 \times 10^{10}$  to  $F = 7 \times 10^{10}$  ph/s. The highest flux of  $F = 7 \times 10^{10}$  ph/s corresponds to the full beam and the curves do not show any significant changes with increasing flux. The decorrelation rate  $\Gamma(q)$  against  $q^2$  is shown in the inset along with the linear fits of  $\Gamma = D q^2$  (solid lines), where  $D$  is

the diffusion coefficient and is the slope of the curves. The fit describes well the data for the probed  $q$ -range, indicating that at these conditions we observe Brownian diffusion. The slope is slightly increased for the highest flux of  $7 \times 10^{10}$  ph/s compared to  $1.6 \times 10^{10}$  ph/s 22.5% of transmission providing diffusion coefficient of  $D = (4.76 \pm 0.05) \times 10^{-3} \text{ nm}^2/\mu\text{s}$  and  $D = (4.25 \pm 0.07) \text{ nm}^2/\mu\text{s}$  respectively. This minor difference is attributed to a heating effect of less than  $\approx 0.5$  K by the X-ray beam, by calculating the corresponding temperature-induced increased solvent viscosity.

To investigate possible effects of cumulative exposure, the same sample spot was measured repetitively. Fig. S5b shows the intensity autocorrelation functions  $g_2(q, t)$  at momentum transfer  $q = 0.1 \text{ nm}^{-1}$  at  $T = 220$  K are displayed for four repetitions and the extracted decorrelation rate  $\Gamma(q)$  (shown in the inset) as a function of the squared momentum transfer  $q^2$ . Based on these results, we conclude that repeated exposure at the same sample spot does not induce any significant changes in the decorrelation rate. However, only the first repetition is used in the analysis presented in the paper.

These results indicate that we do not observe any significant beam-induced effects under these experimental conditions. This could be due to the presence of glycerol which acts like a radical scavenger combined with the low temperatures which mitigate such effects.<sup>4</sup> In addition, the high coherence of ESRF allows for XPCS measurements with reduced flux density due to the relatively large beam used here.

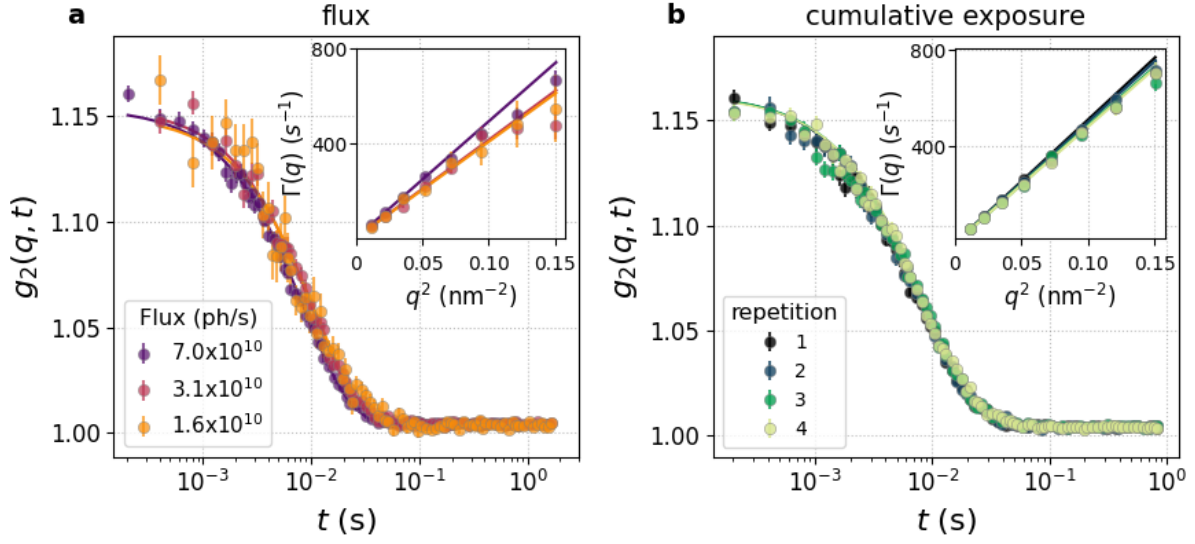

Fig. S5: Flux-dependent X-ray Photon Correlation Spectroscopy (XPCS) measurements. (a) Intensity autocorrelation functions  $g_2(q, t)$  at  $T = 220$  K for different flux conditions at  $q = 0.1$  nm $^{-1}$ , fitted with an exponential function (solid lines). In the inset is shown the decorrelation time  $\Gamma(q)$  as a function of the squared momentum transfer  $q^2$  along with a linear fit (solid line). (b) Cumulative exposure  $g_2(q, t)$  measurements at  $T = 220$  K at momentum transfer  $q = 0.1$  nm $^{-1}$  and flux  $F = 7 \times 10^{10}$  ph/s, fitted with an exponential function (solid line). In the inset is decorrelation time  $\Gamma(q)$  as a function of  $q^2$  along with a linear fit (solid line). The error bars are estimated from the exponential fit.

## References

- (1) Dallari, F.; Martinelli, A.; Caporaletti, F.; Sprung, M.; Baldi, G.; Monaco, G. Stochastic atomic acceleration during the X-ray-induced fluidization of a silica glass. *Proc. Natl. Acad. Sci. U.S.A.* **2023**, *120*, e2213182120.
- (2) Chushkin, Y.; Gulotta, A.; Roosen-Runge, F.; Pal, A.; Stradner, A.; Schurtenberger, P. Probing Cage Relaxation in Concentrated Protein Solutions by X-Ray Photon Correlation Spectroscopy. *Phys. Rev. Lett.* **2022**, *129*, 238001.
- (3) Reiser, M. et al. Resolving molecular diffusion and aggregation of antibody proteins with megahertz X-ray free-electron laser pulses. *Nat. Commun.* **2022**, *13*, 1–10.
- (4) Kuwamoto, S.; Akiyama, S.; Fujisawa, T. Radiation damage to a protein solution, de-

tected by synchrotron X-ray small-angle scattering: dose-related considerations and suppression by cryoprotectants. *J. Synchrotron Radiat.* **2004**, *11*, 462–468.
